# Supplementary material for: Measurement of Z/gamma*+jet+X angular distributions in ppbar collisions at sqrt{s}=1.96 TeV
Source: arXiv:0907.4286 source file (2009-12-14)
Supplement: Supplementary file 1 [file additional.tex]

\clearpage
\section{Tables of Results}
Tables \ref{tab:fulldphi25} to \ref{tab:fullyb45} contain the normalised differential cross sections, $1/\sigma\times d\sigma/d X$, for the three angular variables \dphi, \adrap\ and \ayboost. 
For each bin we present the bin edges, bin average (defined in the main text), measured value, statistical uncertainty, uncorrelated systematic uncertainty, and the systematic uncertainties from these sources, which are correlated across all bins and all distributions: 
\begin{enumerate}
\item $\Delta \phi, \Delta y, y_{\text{boost}}$ reweighting uncertainty; 
\item Jet y reweighting uncertainty; 
\item \Z\ p$_{\text{T}}$\ reweighting uncertainty; 
\item Jet p$_{\text{T}}$\ reweighting uncertainty; 
\item Data overlay on simulation uncertainty; 
\item Muon 1/p$_{\text{T}}$\ resolution uncertainty; 
\item Muon identification efficiency uncertainty; 
\item Jet identification efficiency uncertainty;
\item Jet energy resolution uncertainty; 
\item Jet energy scale uncertainty.
\end{enumerate}

\input supplemental.tex
